# Supplementary material for: Convolutional Neural Opacity Radiance Fields
Source: arXiv:2104.01772 source file (2021-04-05)
Supplement: Supplementary file 1 [file appendix.tex]

\section{Appendix}

\begin{figure*}[!t]
\centering
  \includegraphics[width=1.0\linewidth]{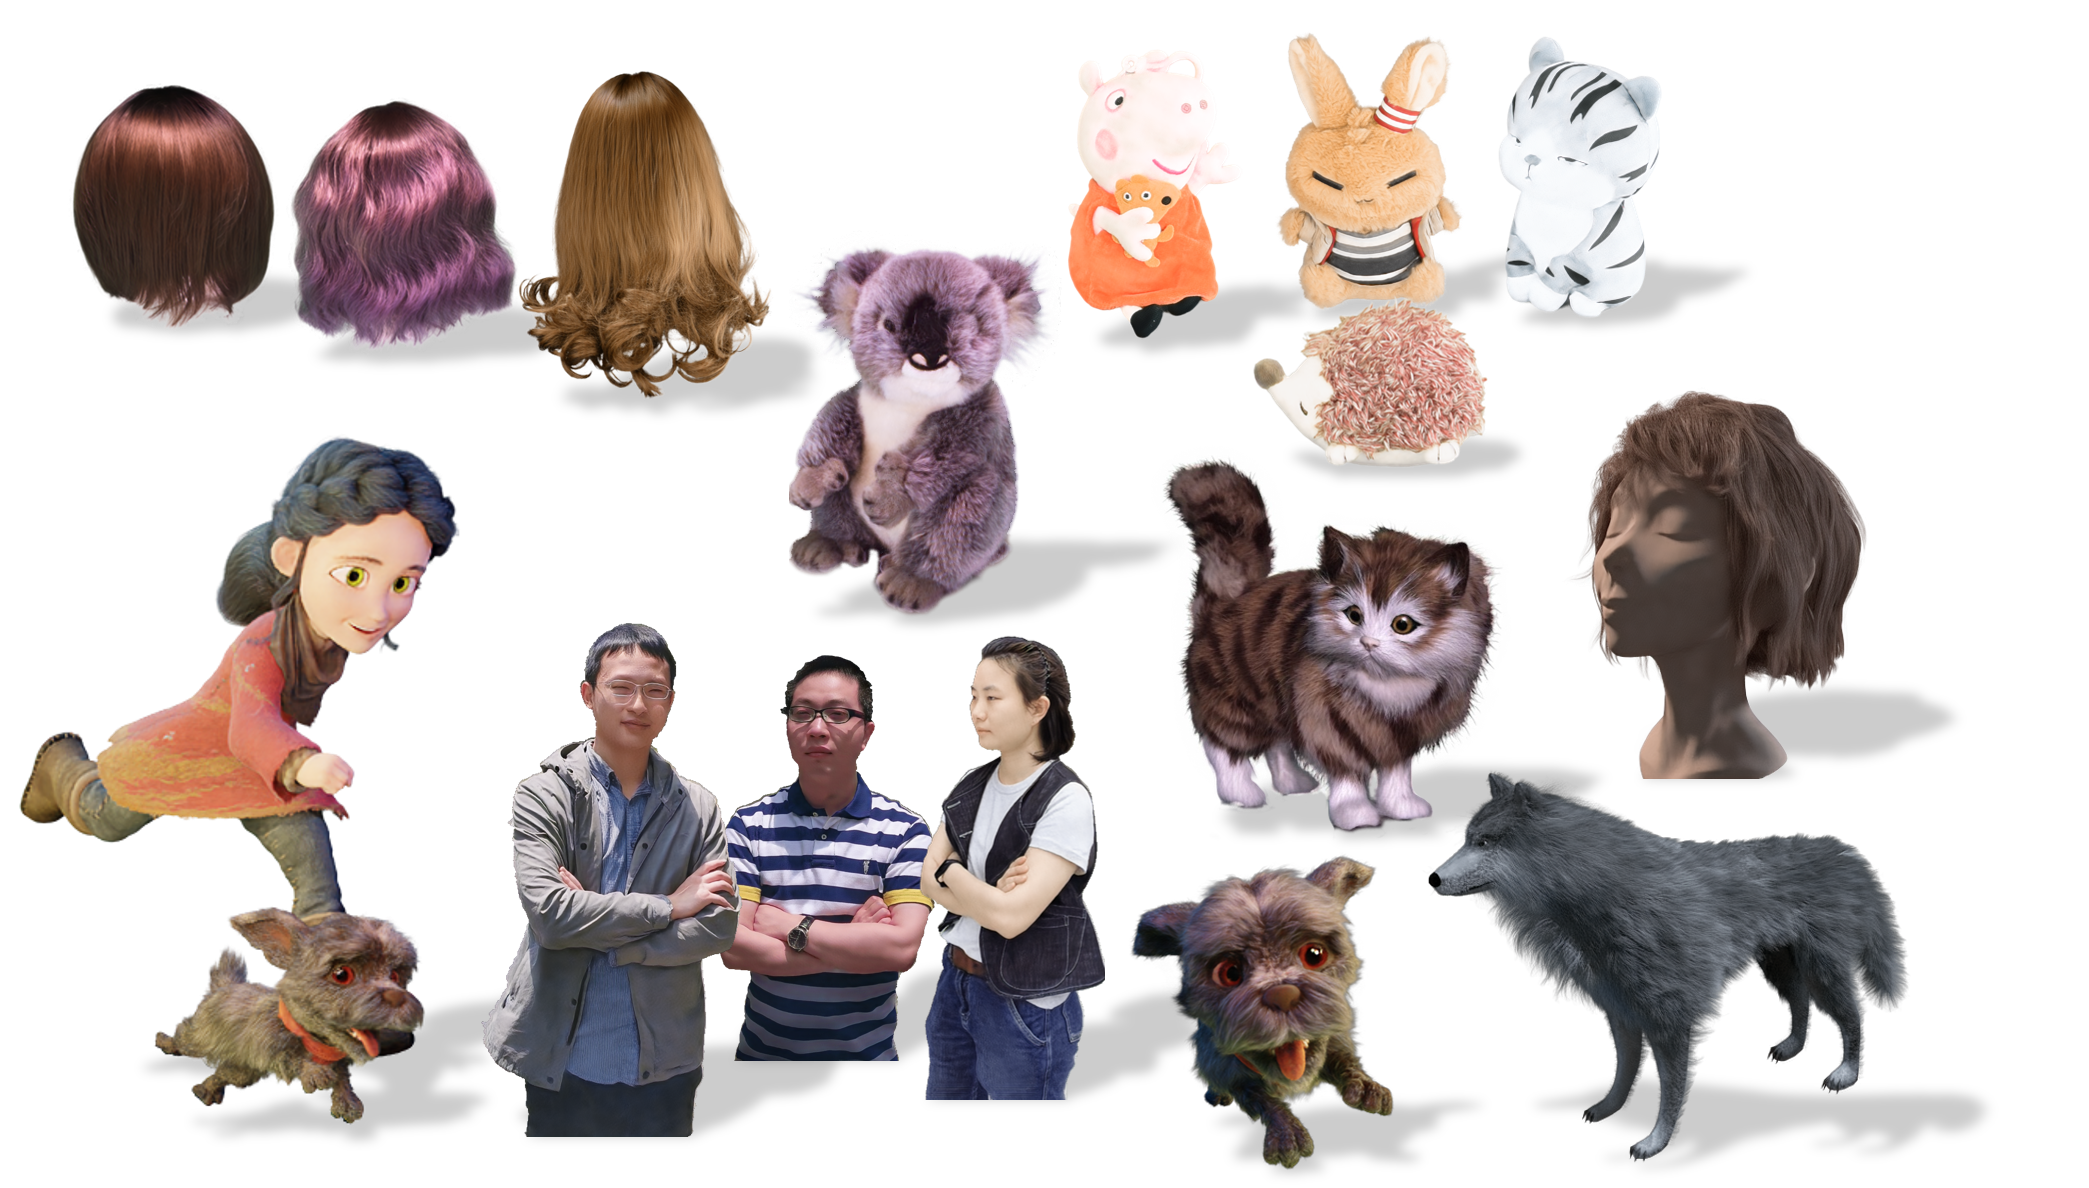}
  \caption{Gallery}
  \label{fig:gallery}
\end{figure*}
